# Supplementary material for: The Software Observatory: aggregating and analysing software metadata for trend computation and FAIR assessment
Source: arXiv:2510.05705 ancillary file (2025-10-07)
Supplement: Supplementary file 1 [file The_Software_Observatory_Supplementary_materials.pdf]

## Supplementary Materials

This document provides additional figures and details supporting the main article: *"The Software Observatory: aggregating and analysing software metadata for trend computation and FAIR assessment"*, Eva Martín del Pico 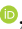, Josep Lluís Gelpí 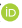 and Salvador Capella-Gutiérrez 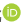, 2025.

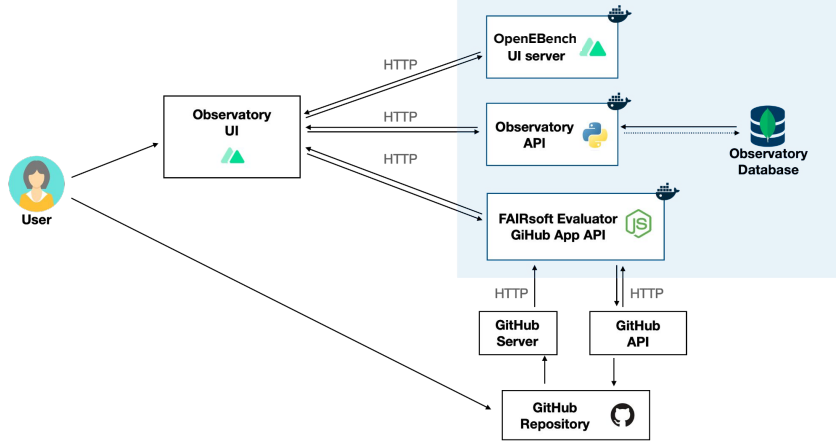

**Figure S1:** System architecture of the Software Observatory within the OpenEBench platform. The Observatory is implemented as a single-page application embedded in the OpenEBench (OEB) web platform. The user interface—referred to in this paper as the “Observatory interface”—is rendered by the OEB UI server, built with NuxtJS. This interface communicates via HTTP with two backend services: (1) the Observatory API (Python/FastAPI), which handles data ingestion, scoring, and metadata integration; and (2) the FAIRsoft Evaluator GitHub App API (NodeJS/Express), which manages authenticated interactions with GitHub. GitHub authentication and permissions are handled using two GitHub Apps (i.e., registered integration entities, not visual components): the metadata extraction app retrieves metadata from public repositories, while the contribution app creates pull requests to add or update structured metadata such as `CITATION.cff` files. All services are containerized using Docker, and the GitHub App API is configured through environment variables that include App IDs and private keys. This modular architecture enables secure, scalable, and semi-automated FAIR metadata workflows within the Software Observatory.

| Data Source                  | Raw records | Collection Method       | Access Method  | Metadata Format                     |
|------------------------------|-------------|-------------------------|----------------|-------------------------------------|
| <a href="#">bio.tools</a>    | 36,665      | OpenEBench <sup>1</sup> | REST API       | Structured (JSON)                   |
| <a href="#">GitHub</a>       | 3,918       | GitHub APIs             | REST/GraphQL   | Structured (JSON)                   |
| <a href="#">Bioconda</a>     | 10,215      | Bioconda recipes repo   | Git            | Structured (YAML)                   |
| <a href="#">Bioconductor</a> | 3,499       | Bioconductor packages   | Git            | Structured (DESCRIPTION + CITATION) |
| <a href="#">Galaxy</a>       | 1,543       | OpenEBench <sup>1</sup> | REST API       | Structured (JSON)                   |
| <a href="#">ToolShed</a>     | 7,095       | ToolShed repositories   | Mercurial (hg) | Structured (XML)                    |
| <a href="#">SourceForge</a>  | 3,007       | Web scraping            | Web scraping   | Semi-structured (HTML)              |

**Table S1:** Overview of metadata sources used in the Software Observatory.

<sup>1</sup> OpenEBench technical monitoring retrieves metadata from the [ELIXIR Software Ecosystem](#).

| Component                                                                         | Repository URL                                                                                                                                                              |
|-----------------------------------------------------------------------------------|-----------------------------------------------------------------------------------------------------------------------------------------------------------------------------|
| <b>Metadata Importers</b>                                                         |                                                                                                                                                                             |
| bio.tools importer                                                                | <a href="https://gitlab.bsc.es/inb/elixir/software-observatory/oepb-tools-importer">https://gitlab.bsc.es/inb/elixir/software-observatory/oepb-tools-importer</a>           |
| GitHub importer                                                                   | <a href="https://github.com/inab/github-importer">https://github.com/inab/github-importer</a>                                                                               |
| Bioconda importer                                                                 | <a href="https://gitlab.bsc.es/inb/elixir/software-observatory/bioconda-recipes">https://gitlab.bsc.es/inb/elixir/software-observatory/bioconda-recipes</a>                 |
| Bioconductor importer                                                             | <a href="https://gitlab.bsc.es/inb/elixir/software-observatory/bioconductor-importer-v2">https://gitlab.bsc.es/inb/elixir/software-observatory/bioconductor-importer-v2</a> |
| Galaxy importer                                                                   | <a href="https://gitlab.bsc.es/inb/elixir/software-observatory/oepb-tools-importer">https://gitlab.bsc.es/inb/elixir/software-observatory/oepb-tools-importer</a>           |
| ToolShed importer                                                                 | <a href="https://gitlab.bsc.es/inb/elixir/software-observatory/toolshed-importer">https://gitlab.bsc.es/inb/elixir/software-observatory/toolshed-importer</a>               |
| SourceForge importer                                                              | <a href="https://gitlab.bsc.es/inb/elixir/software-observatory/sourceforge-importer">https://gitlab.bsc.es/inb/elixir/software-observatory/sourceforge-importer</a>         |
| <b>Processing and Integration Pipeline</b>                                        |                                                                                                                                                                             |
| Transformation, normal-<br>ization, enrichment, inte-<br>gration and calculations | <a href="https://github.com/inab/research-software-etl">https://github.com/inab/research-software-etl</a>                                                                   |
| License normalisation                                                             | <a href="https://github.com/inab/licenses-mapping">https://github.com/inab/licenses-mapping</a>                                                                             |
| <b>User-Facing and Backend Services</b>                                           |                                                                                                                                                                             |
| OpenEBench UI                                                                     | <a href="https://github.com/inab/openEBench-nuxt">https://github.com/inab/openEBench-nuxt</a>                                                                               |
| Observatory API                                                                   | <a href="https://github.com/inab/observatory-api">https://github.com/inab/observatory-api</a>                                                                               |
| FAIRsoft GitHub API                                                               | <a href="https://github.com/inab/github-metadata-api">https://github.com/inab/github-metadata-api</a>                                                                       |

**Table S2:** List of Software Observatory components grouped by function, with links to their respective repositories.

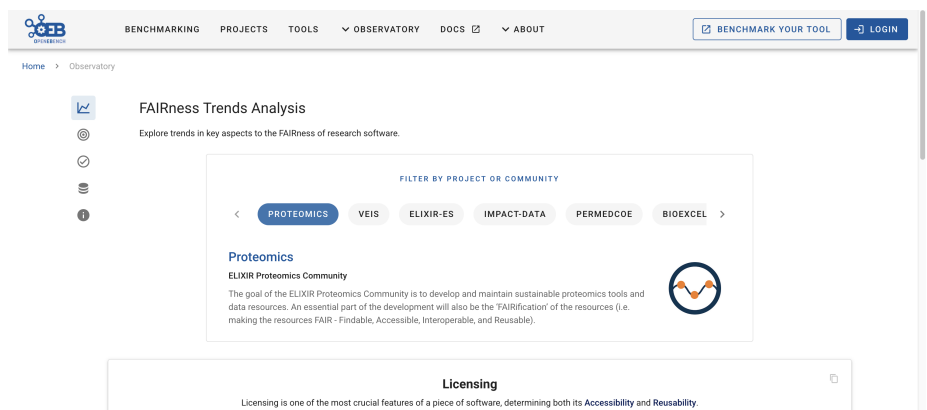

**Figure S2:** FAIRness Trends Analysis interface of the Software Observatory, shown here for the ELIXIR Proteomics Community. A key feature is the collection selector at the top, which allows filtering by project or community (e.g., VEIS, ELIXIR-ES, Impact-Data). This selector is consistently available across the Trends, Data, and FAIRsoft Scoreboard sections, facilitating focused analysis of software FAIRness within specific domains.

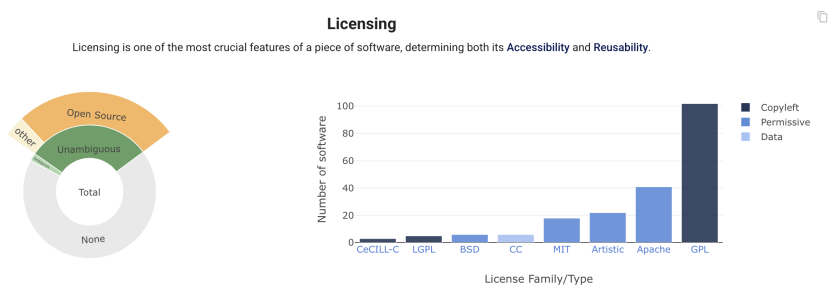

**Figure S3:** "Licensing" panel of the FAIRness Trends Analysis interface of the Software Observatory, shown for the ELIXIR Proteomics Community.

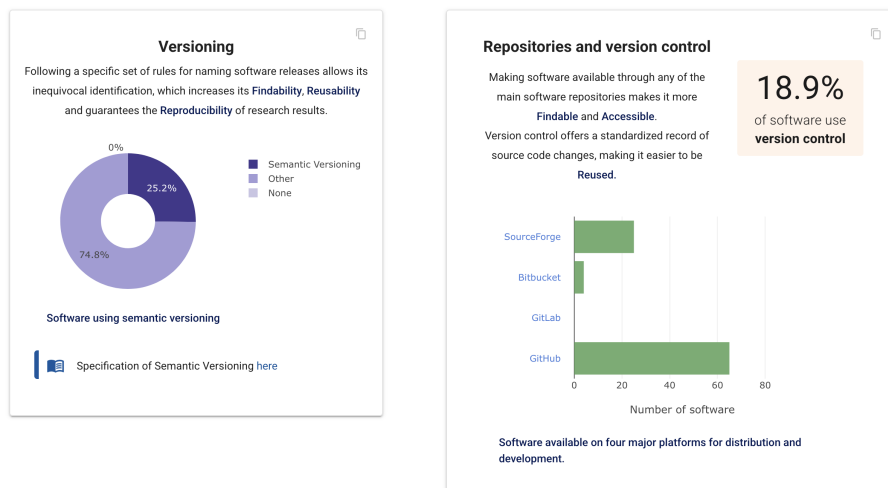

**Figure S4:** "Versioning" and "Repositories and Version control" panels of the FAIRness Trends Analysis interface of the Software Observatory, shown for the ELIXIR Proteomics Community.

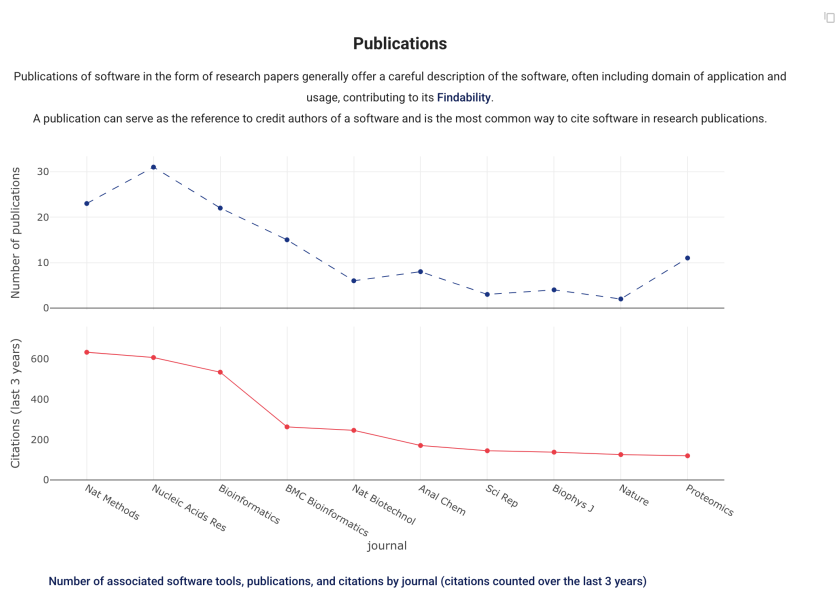

**Figure S5:** "Publication" panel of the FAIRness Trends Analysis interface of the Software Observatory, shown for the ELIXIR Proteomics Community.

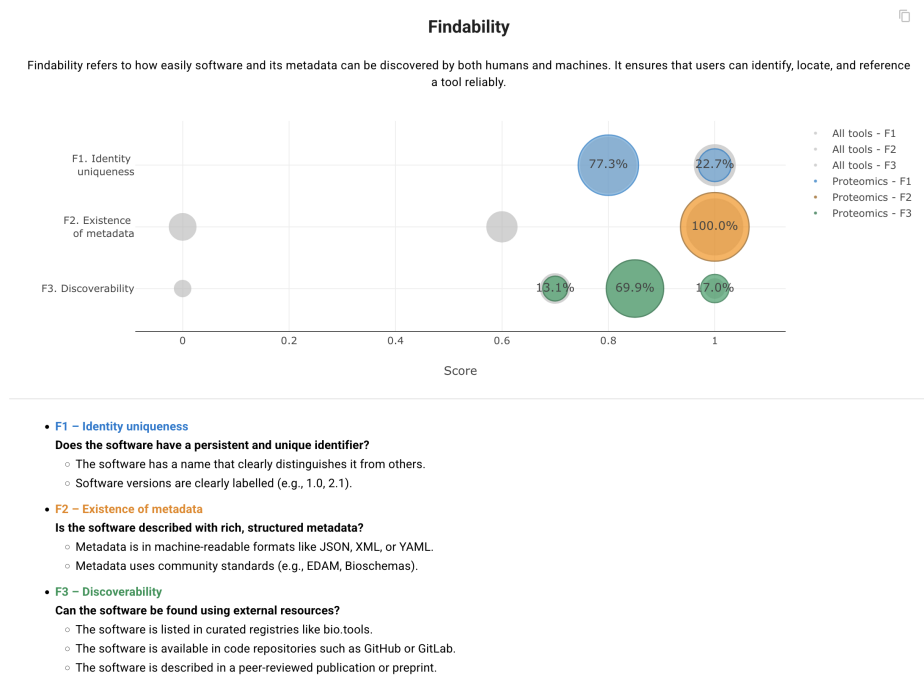

**Figure S6:** "Findability" panel of the FAIRsoft Indicator Scoreboard interface of the Software Observatory, shown for the ELIXIR Proteomics Community.

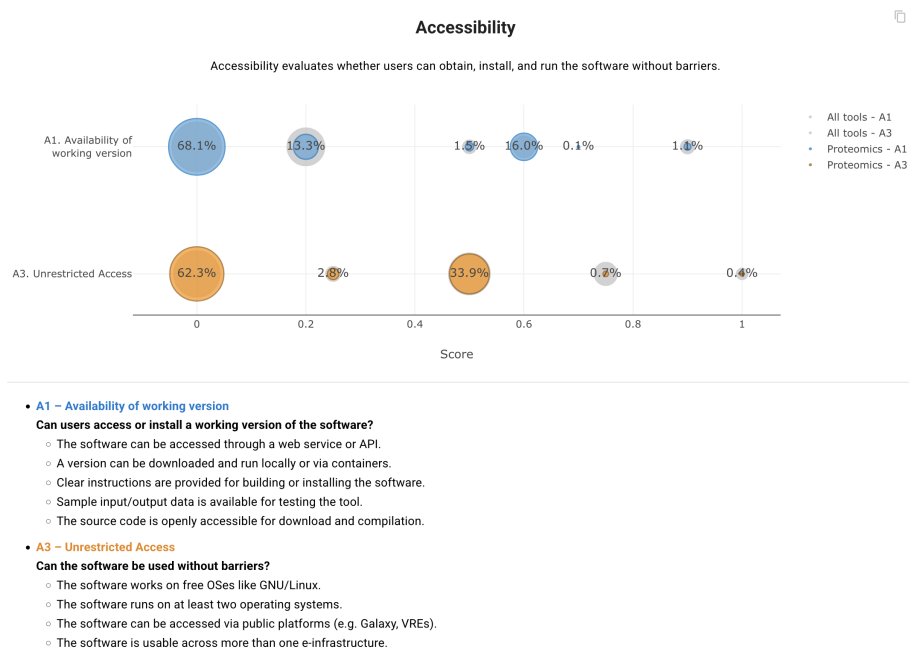

**Figure S7:** "Accessibility" panel of the FAIRsoft Indicator Scoreboard interface of the Software Observatory, shown for the ELIXIR Proteomics Community.

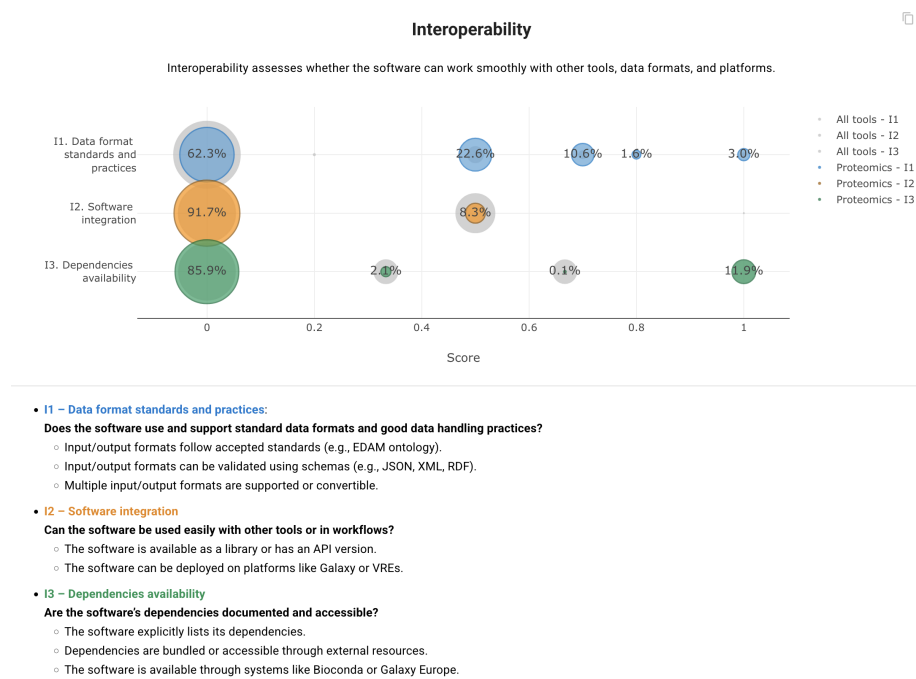

**Figure S8:** "Interoperability" panel of the FAIRsoft Indicator Scoreboard interface of the Software Observatory, shown for the ELIXIR Proteomics Community.

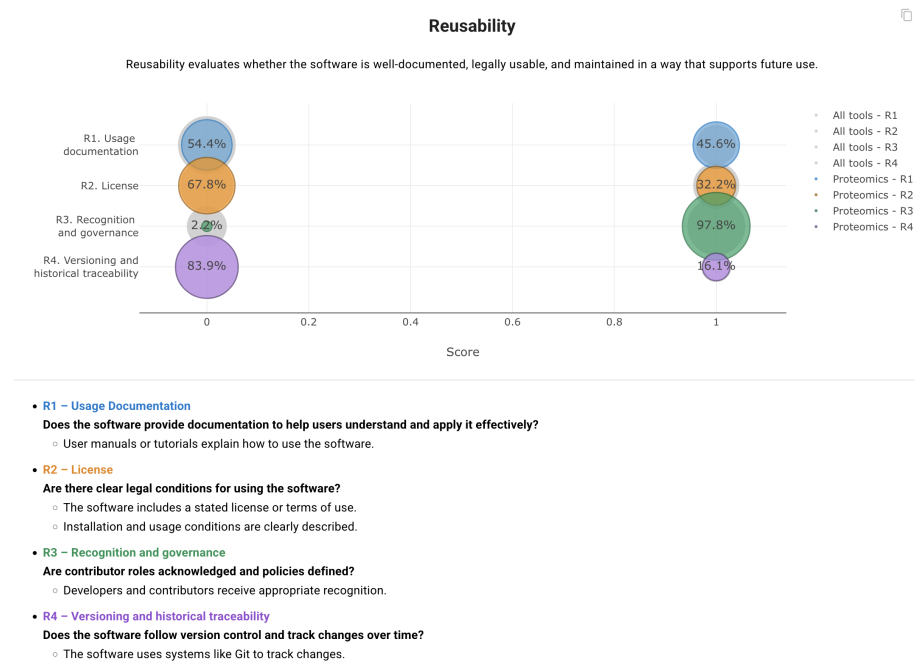

**Figure S9:** "Reusability" panel of the FAIRsoft Indicator Scoreboard interface of the Software Observatory, shown for the ELIXIR Proteomics Community.

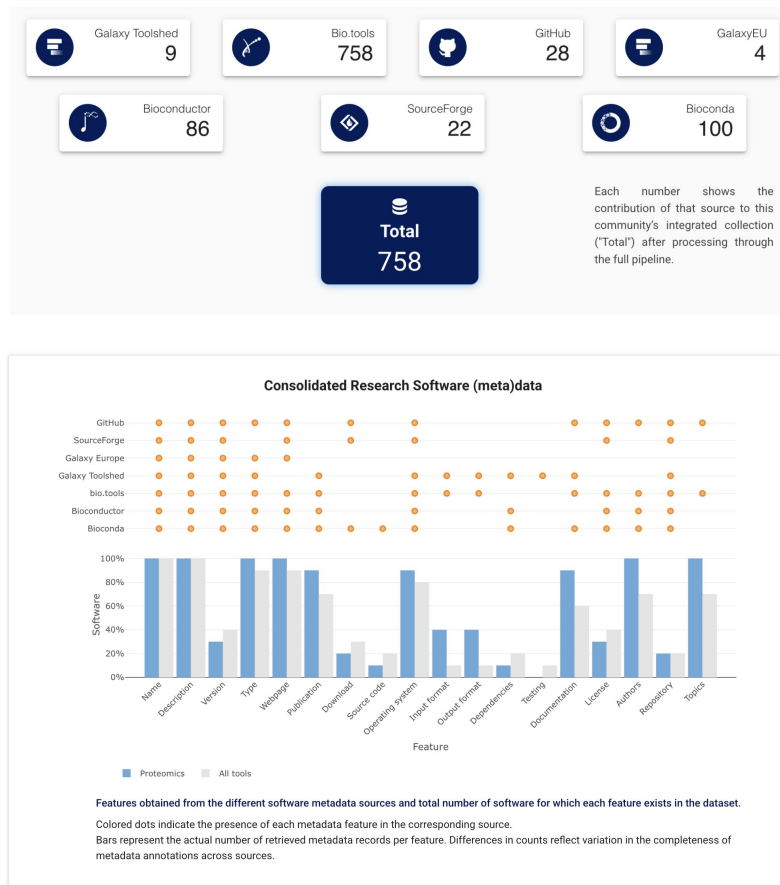

**Figure S10: Integrated metadata overview for the ELIXIR Proteomics Community in the Software Observatory.** This composite view illustrates the software integration and metadata coverage achieved by the Software Observatory. The top section displays the number of software tools contributed by each metadata source after harmonization. The bottom section presents metadata coverage across sources for key features such as version, license, and documentation. Dots indicate availability of metadata fields, while bars reflect the number of entries in the final dataset containing each feature. Together, these panels highlight both the scale and variability of metadata integration, which the FAIRsoft Evaluator addresses to support FAIRness assessments.

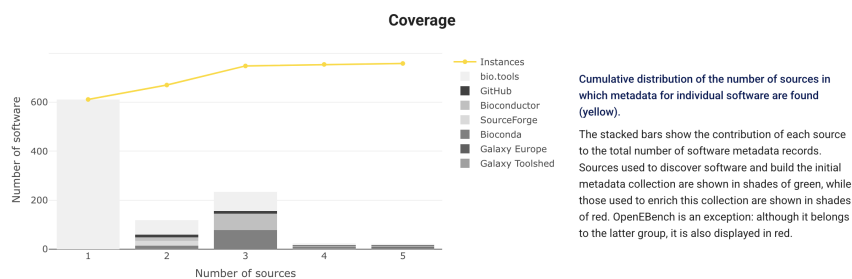

**Figure S11:** "Coverage" panel of the Data interface of the Software Observatory.

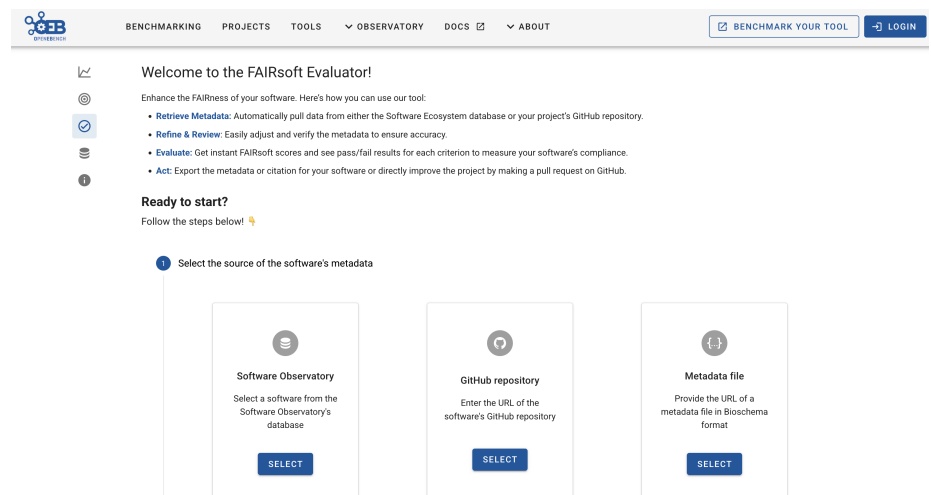

**Figure S12:** Initial page of the FAIRsoft Evaluator within the Software Observatory. This interface guides users through the evaluation process by first selecting the source of the software's metadata. Users can choose to retrieve metadata from the Software Observatory's database, a GitHub repository, or an external metadata file in maSMP format [1]. The page also outlines the four main steps of the tool: Retrieve, Refine, Evaluate, and Act.

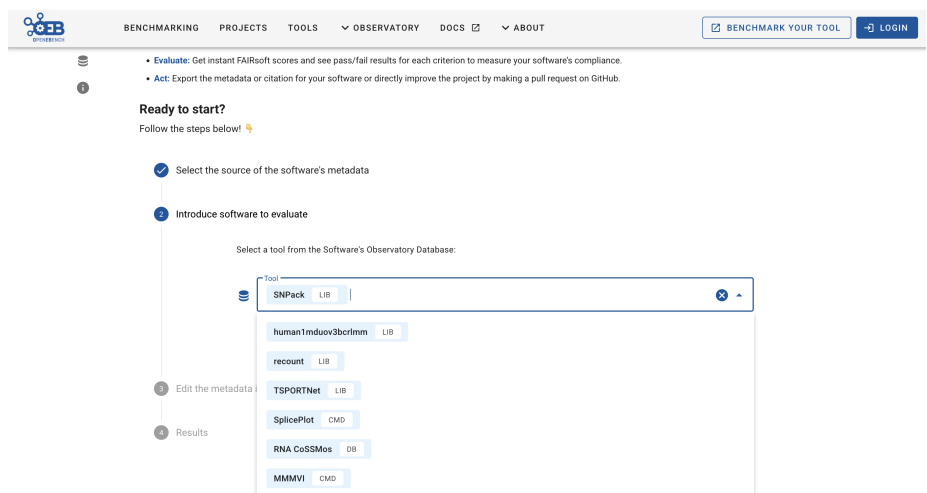

**Figure S13:** Second step of the FAIRsoft Evaluator within the Software Observatory: selecting a software entry to evaluate. After choosing the metadata source, users are prompted to select a specific software tool from the Observatory's database. The interface supports search and auto-completion, and each entry is labeled by type (e.g., LIB for library, CMD for command-line tool), facilitating targeted evaluation of diverse software categories.



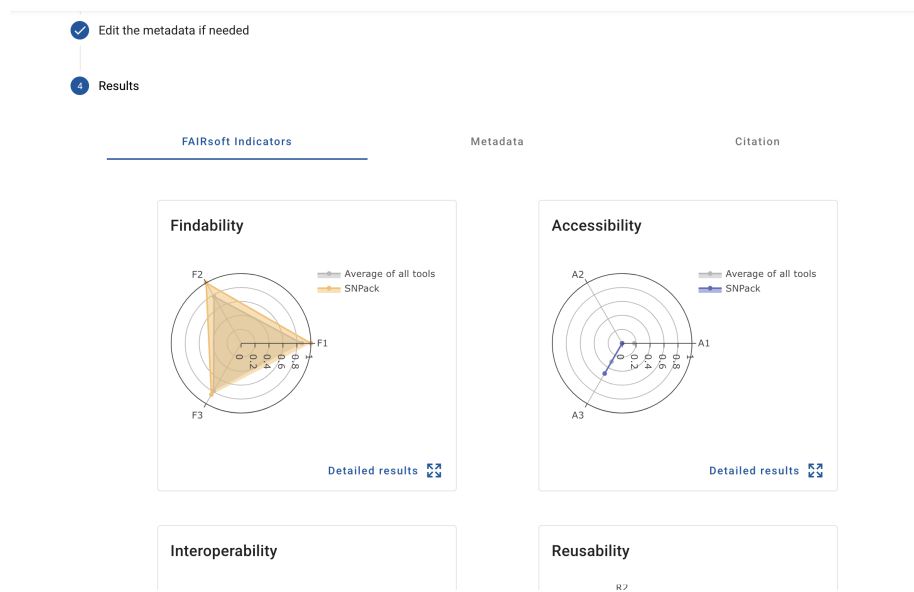

**Figure S15:** Summary of results in the FAIRsoft Evaluator. Radar plots visualize performance across the sub-indicators for each FAIR principle. Findability and Accessibility are visible in the image.

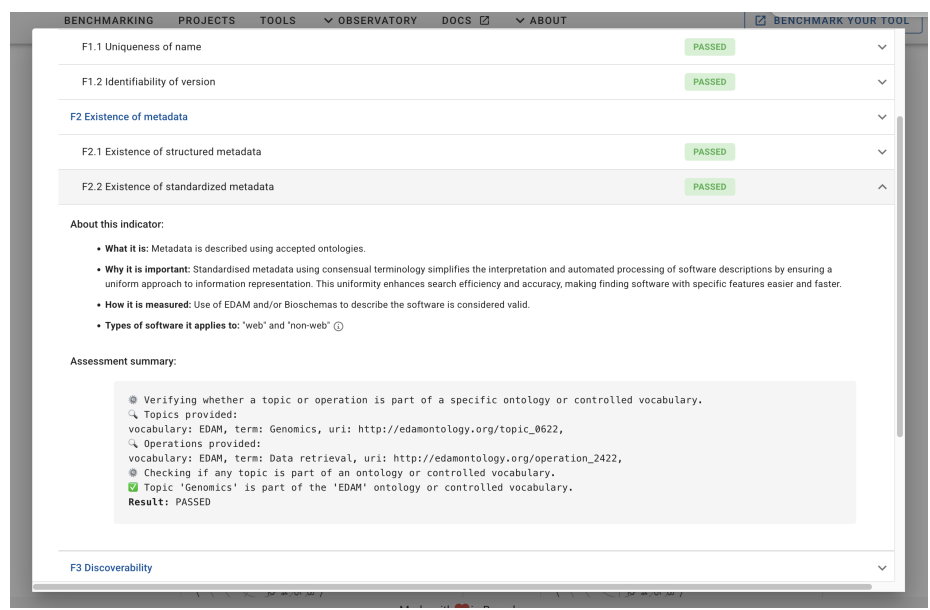

**Figure S16:** Detail of Findability results in the FAIRsoft Evaluator, focusing on indicator F2: Existence of metadata. This view allows users to understand not only whether their software passes or fails a given indicator, but also why. Each indicator includes a clear definition, an explanation of its relevance, and a description of how it is assessed. In this example, the software passes because it uses standardised vocabularies (EDAM terms) to describe both topics and operations. By making the evaluation logic explicit, this interface helps users judge the relevance of each indicator for their specific context and offers concrete guidance on how to improve their FAIRness score.

## References

- [1] Giraldo Olga, Geist Lukas, Quiñones Nelson, Solanki Dhwani, Rebholz-Schuhmann Dietrich, and Castro Leyla Jael. Machine-actionable Software Management Plan Ontology (maSMP Ontology). April 2023.
